# Supplementary material for: LipCoder: Voice-Enabled Coding Toolkit
Source: arXiv:2608.30793 source file (2026-08-31)
Supplement: Supplementary file 1 [file appendix-tagged.tex]

% Accessible (tagged) build of the APPENDICES ONLY (supplementary material).
% Compile THIS file to produce the tagged supplementary PDF:
%   pdflatex appendix-tagged  ->  bibtex appendix-tagged  ->  pdflatex x2
% \DocumentMetadata must appear before \documentclass, hence this wrapper.
%
% Everything else follows from \buildmode; see the BUILD MODE block in main.tex,
% which also starts the table counter at 3 so the appendix keeps its
% full-document table numbers (Tables 4-9) and reads main-labels.tex so that
% references into the main paper (Section 5, Tables 1-3) still resolve.
\DocumentMetadata{
  lang        = en-US,
  pdfversion  = 1.7,
  testphase   = {phase-III, table, math, firstaid},
}
\def\buildmode{appendix}
\input{main.tex}
